# Supplementary material for: Active learning of reactive Bayesian force fields: Application to heterogeneous hydrogen-platinum catalysis dynamics
Source: arXiv:2106.01949 ancillary file (2021-06-03)
Supplement: Supplementary file 1 [file Supplementary_Information.pdf]

Supplementary Information for

# Active learning of reactive Bayesian force fields: Application to heterogeneous hydrogen-platinum catalysis dynamics

Jonathan Vandermause

*Department of Physics, Harvard University, Cambridge, Massachusetts 02138, USA and John A. Paulson School of Engineering and Applied Sciences, Harvard University, Cambridge, MA 02138, USA*

Yu Xie

*John A. Paulson School of Engineering and Applied Sciences, Harvard University, Cambridge, MA 02138, USA*

Jin Soo Lim and Cameron J. Owen

*Department of Chemistry and Chemical Biology, Harvard University, Cambridge, MA 02138, USA*

Boris Kozinsky

*John A. Paulson School of Engineering and Applied Sciences, Harvard University, Cambridge, MA 02138, USA and Bosch Research, Cambridge, MA 02139, USA*

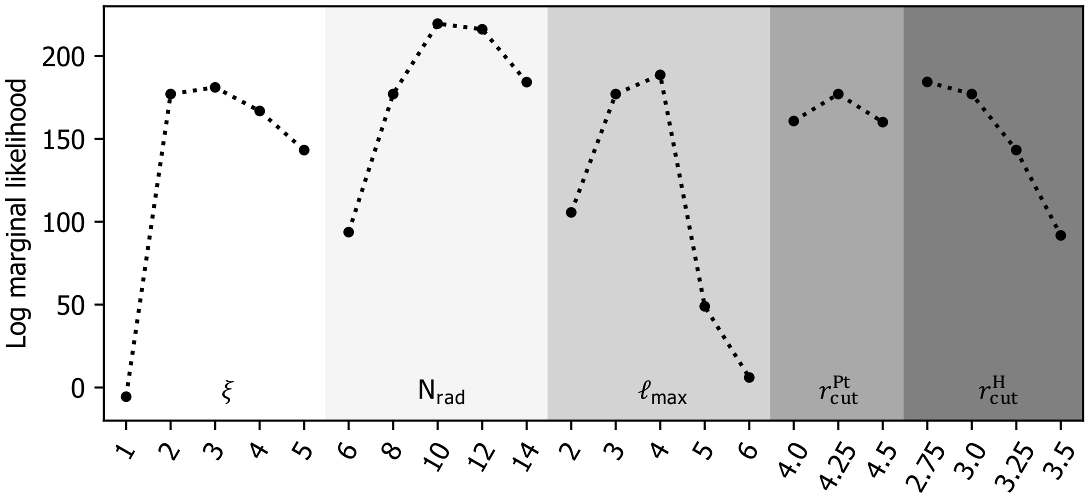


FIG. 1. The SGP likelihood for various integer kernel powers $\xi$, basis set expansion parameters $N_{\mathrm{rad}}$ and $\ell_{\mathrm{max}}$, and model cutoffs $r_{\mathrm{cut}}^{\mathrm{Pt}}$ (denoting the Pt-Pt cutoff) and $r_{\mathrm{cut}}^{\mathrm{H}}$ (denoting the Pt-H and H-H cutoffs, which were set equal to each other). The likelihood was evaluated with five structures from the Pt/H training simulation in the training set of the SGP.

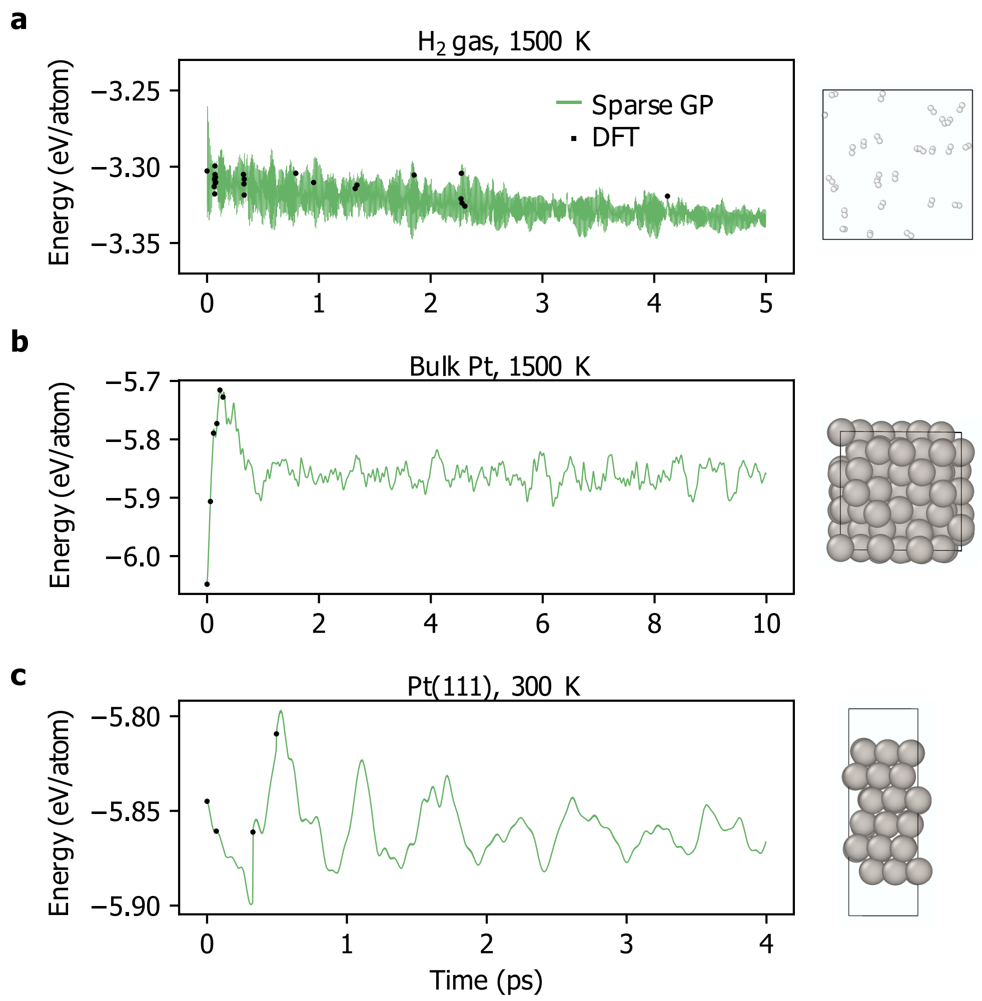


FIG. 2. Potential energy versus time for three of the four on-the-fly training simulations reported in the main text: (a) $H_2$ gas at 1500 K, (b) bulk fcc platinum at 1500 K, and (c) a six-layer Pt(111) slab at 300 K. Example structures from the simulations are shown on the right.

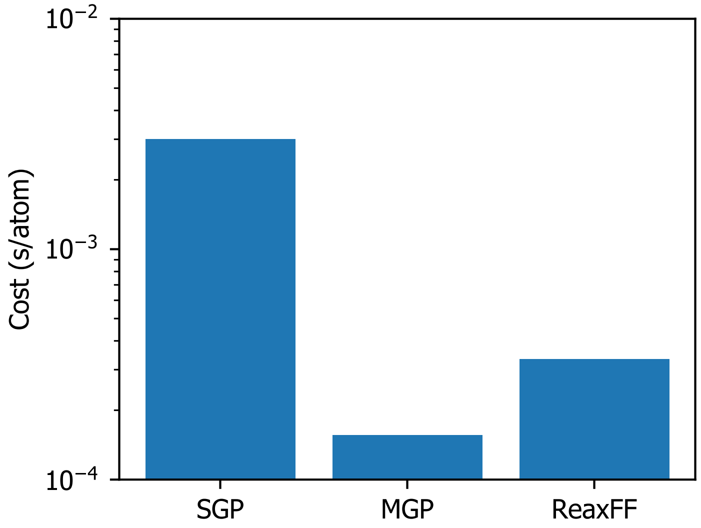


FIG. 3. Prediction cost in seconds per atom with the SGP, the equivalent mapped model implemeneted in LAMMPS (labelled MGP), and the Pt/H ReaxFF force field. A single cpu was used to evaluate the models on the same structure, which consisted of a single H adsorbate on a six-layer 3x3 Pt(111) slab.

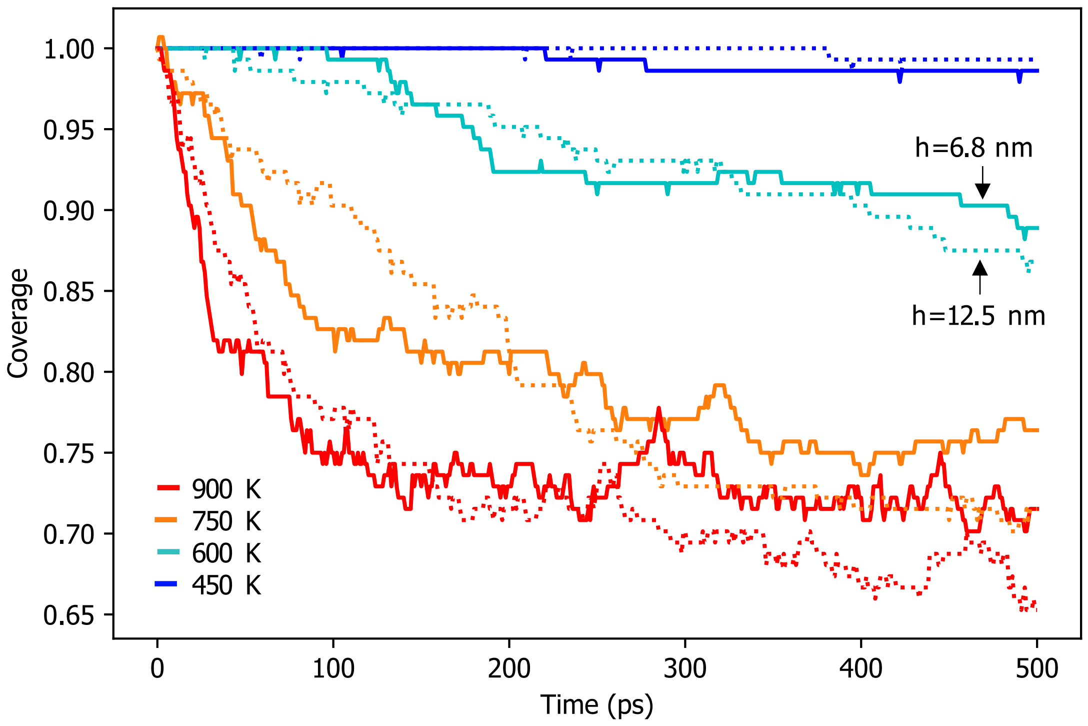


FIG. 4. Surface coverage as a function of time for the production MD simulations reported in the main text.

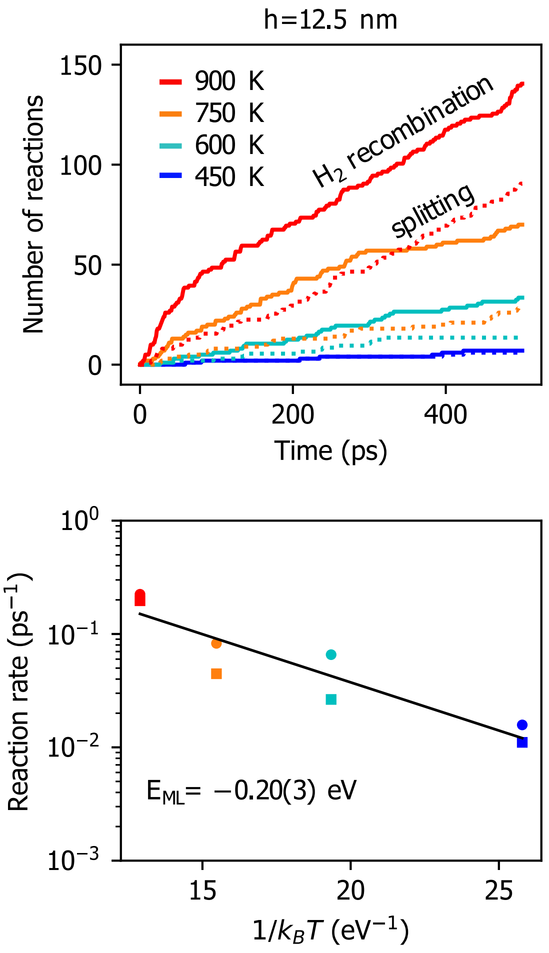


FIG. 5. Reaction rates (top) and Arrhenius plot (bottom) for simulations conducted with the 12.5-nm box height.
